# Supplementary material for: Audio-FLAN: An Instruction-Following Dataset for Unified Audio Understanding and Generation of Speech, Music, and Sound
Source: arXiv:2502.16584 source file (2026-06-07)
Supplement: Supplementary file 1 [file qwen2-tuning-results-appendix.tex]

\onecolumn
\begin{longtable}[hbtp]{p{4.6cm}<{\raggedright}p{4.5cm}<{\raggedright}p{4.5cm}<{\raggedright}}   % 设置列宽，p{width}表示自动换行
\caption{Evaluation results of Qwen2 tuning results. \lmxue{select some tasks in main paper, and move all tasks to appendix. } }  % 表格标题
\label{tab:qwen2_tuning_result}  % 表格标签，用于引用
\\  % 用来初始化表格
\hline
\textbf{Tasks} & \textbf{Results after tuning} & \textbf{Results w/o tuning}\\
\hline
\endfirsthead  % 每页表头部分
\multicolumn{3}{|c|}{\textit{Continued from the previous page}} \\  % 跨页表头
\hline
\textbf{Tasks} & \textbf{Results after tuning} & \textbf{Results w/o tuning}\\
\hline
\endhead  % 继续表头部分
\hline
\endfoot  % 每页的表尾部分
\hline
\endlastfoot  % 最后一页的表尾部分

% \toprule
    % Tasks & Results after tuning & Results w/o tuning  \\  % 表头
    % \midrule % Speech Tasks
    % Age Recognition & \textit{MAE}=3.7092, \textit{MSE}=22.9723 & \textit{MAE}=5.3288, \textit{MSE}=47.1621 \\  % 行数据
    % Speech-to-text Translation & \textit{WER}=1.0768, \textit{BLEU-1}=0.2746, \textit{BLEU-4}=0.0928, \textit{METEOR}=0.3055, ROUGE\_L=0.2198, \textit{CIDEr}=0.8853 & \textit{WER}=4.5813, \textit{BLEU-1}=0.0594, \textit{BLEU-4}=0.0097, \textit{METEOR}=0.1645, \textit{ROUGE\_L}=0.0668, \textit{CIDEr}=0.1171\\
    % Speech Caption & \textit{BLEU-1}=0.6508, \textit{BLEU-4}=0.3970, \textit{METEOR}=0.3908, \textit{ROUGE\_L}=0.5717, \textit{CIDEr}=0.8700 & \textit{BLEU-1}=0.0830, \textit{BLEU-4}=0.0020, \textit{METEOR}=0.0973, \textit{ROUGE\_L}=0.0627, \textit{CIDEr}=0.0077\\
    Automatic Speech Recognition & \textit{WER}=0.7021 & \textit{WER}=1.1941 \\
    Gender Recognition & \textit{ACC}=0.9834 & \textit{ACC}=0.8773\\
    Dialect Identification & \textit{ACC}=0.7264 & \textit{ACC}=0.6644\\
    Emotion Recognition (speech) & \textit{ACC}=0.8260 & \textit{ACC}=0.3801\\
    % Language Identification & \textit{ACC}=0.6270 & \textit{ACC}=0.3916\\
    % Deepfake Detection & \textit{ACC}=0.5447	& \textit{ACC}=0.1835\\
    % Spoken Paragraph Recognition & \textit{EER}=0.4628 & \textit{EER}=0.5093 \\
    % Speaker Verification & \textit{EER}=0.4614 & \textit{EER}=0.5030 \\
    Phonetic Recognition & \textit{WER}=0.1949 & /\\
    Speaker Identification & / & / \\
    \midrule
    Music Genre Recognition & \textit{ACC}=0.2432 & \textit{ACC}=0.0911\\
    Music Genre Recognition & \textit{ACC}=0.1745 & \textit{ACC}=0.0055\\ % (Multiple) 
    Emotion Recognition (music) & \textit{ACC}=0.1756 & \textit{ACC}=0.0683\\
    Artist Identification & \textit{ACC}=0.3681 & /\\
    
    Instrument Classification & \textit{ACC}=0.5723 & / \\ % (Single) 
    % Instrumental Technique Recognition & \textit{ACC}=0.8857 & \textit{ACC}=0.2507\\
    
    Music Tagging & ? & \textit{BLEU-1}=0.0117, \textit{BLEU-4}=0.0034, \textit{METEOR}=0.0932, \textit{ROUGE\_L}=0.0216, \textit{CIDEr}=0.0089 \\ % 核对一下tuning的结果
    % Beat Tracking & \textit{ACC}=0.9138 & / \\
    Key Detection & ACC=0.3601 & ACC=0.1272 \\
    Chord Estimation & \textit{ACC}=0.5015 & \textit{ACC}=0.4464\\
    % Chord Estimation (time-step) & \textit{OLP}=0.4002 & / \\
    Pitch Classification & \textit{ACC}=0.8196 & \textit{ACC}=0.4725 \\ % (Single) 
    Instrument Recognition & \textit{ACC}=0.797 & \textit{ACC}=0.6107\\ % (CHOICE)
    Instrument Recognition & \textit{ACC}=0.3963 & \textit{ACC}=0.2507\\ % (Multiple) 
    
    % Beat-level Pitch Estimation & \textit{ACC}=0.2131 & /\\
    % Beat-level Instrument Recognition & \textit{ACC}=0.5384 & /\\
       
    % Key Comparison & \textit{ACC}=0.9113 & \textit{ACC}=0.1417 \\
    % Tempo Comparison & \textit{ACC}=0.4563 & \textit{ACC}=0.4052 \\
    % Instrument Comparison & \textit{ACC}=0.8597	& \textit{ACC}=0.056 \\
    % Instrumental Technique Comparison & \textit{ACC}=0.9408	& \textit{ACC}=0.1505\\
    
    % Music Caption (CHOICE) & \textit{ACC}=0.6952 & \textit{ACC}=0.3115\\
    % Music Caption & \textit{BLEU-1}=0.4295, \textit{BLEU-4}=0.2612, \textit{METEOR}=0.2347, \textit{ROUGE\_L}=0.4384, \textit{CIDEr}=1.4679 & \textit{BLEU-1}=0.1036, \textit{BLEU-4}=0.0249, \textit{METEOR}=0.0774, \textit{ROUGE\_L}=0.1147, \textit{CIDEr}=0.1165\\
    % Pitch Change Detection & / & / \\

    \midrule
    % Acoustic Scene Classification & \textit{ACC}=0.3666 & \textit{ACC}=0.0634\\
%     Sound Event Sequence Recognition & %\textit{ACC}=0.3733, 
% \textit{BLEU-1}=0.3323, \textit{BLEU-4}=0.3555, \textit{METEOR}=0.2401, \textit{ROUGE\_L}=0.4062, \textit{CIDEr}=1.7834 & %\textit{ACC}=/,
% \textit{BLEU-1}=0.0162, \textit{BLEU-4}=0.0030, \textit{METEOR}=0.0854, \textit{ROUGE\_L}=0.0596, \textit{CIDEr}=0.0692 \\
    Speech, Silence, Music and Noise Classification & \textit{ACC}=0.9757 &	\textit{ACC}=0.6721\\
    % Audio Captioning & \textit{BLEU-1}=0.1285, \textit{BLEU-4}=0.0369, \textit{METEOR}=0.1951, \textit{ROUGE\_L}=0.2886, \textit{CIDEr}=0.9735 & \textit{BLEU-1}=0.0150, \textit{BLEU-4}=0.0027, \textit{METEOR}=0.0904, \textit{ROUGE\_L}=0.0439, \textit{CIDEr}=0.0203\\
    Audio Understanding & \textit{BLEU-1}=0.6971, \textit{BLEU-4}=0.6522, \textit{METEOR}=0.4610, \textit{ROUGE\_L}=0.7461, \textit{CIDEr}=0.0621 & \textit{BLEU-1}=0.1614, \textit{BLEU-4}=0.0225, \textit{METEOR}=0.1497, \textit{ROUGE\_L}=0.1433, \textit{CIDEr}=0.0185 \\
    % Sound Event Detection & \textit{TOR}=0.4197 & \textit{TOR}=0.0341\\
    % Sound Event Detection & ACC=1.0000 & ACC=0.8310 \\ % (3_AudioSet这个任务的所有答案都是yes，需要修改)
    \bottomrule

\end{longtable}
